# Supplementary material for: Extracting Spatiotemporal Demand for Public Transit from Mobility Data
Source: arXiv:2006.03351 ancillary file (2020-06-05)
Supplement: Supplementary file 1 [file Supplementary.pdf]

# Supplementary Information: Extracting Spatiotemporal Demand for Public Transit from Mobility Data

Trivik Verma,<sup>1</sup> Mikhail Sirenko,<sup>1</sup> Itto Kornecki,<sup>2</sup> Scott Cunningham,<sup>3</sup> and Nuno A. M. Araújo<sup>4,5</sup>

<sup>1</sup>*Faculty of Technology, Policy and Management,  
Delft University of Technology, 2628BX Delft, the Netherlands*

<sup>2</sup>*ETH Zürich, Universitätstrasse 16, 8092 Zürich, Switzerland*

<sup>3</sup>*Faculty of Humanities and Social Science, University of Strathclyde,  
18 Richmond Street, Glasgow G1 1XQ, Scotland, United Kingdom*

<sup>4</sup>*Departamento de Física, Faculdade de Ciências,  
Universidade de Lisboa, P-1749-016 Lisboa, Portugal*

<sup>5</sup>*Centro de Física Teórica e Computacional, Faculdade de Ciências,  
Universidade de Lisboa, 1749-016 Lisboa, Portugal*

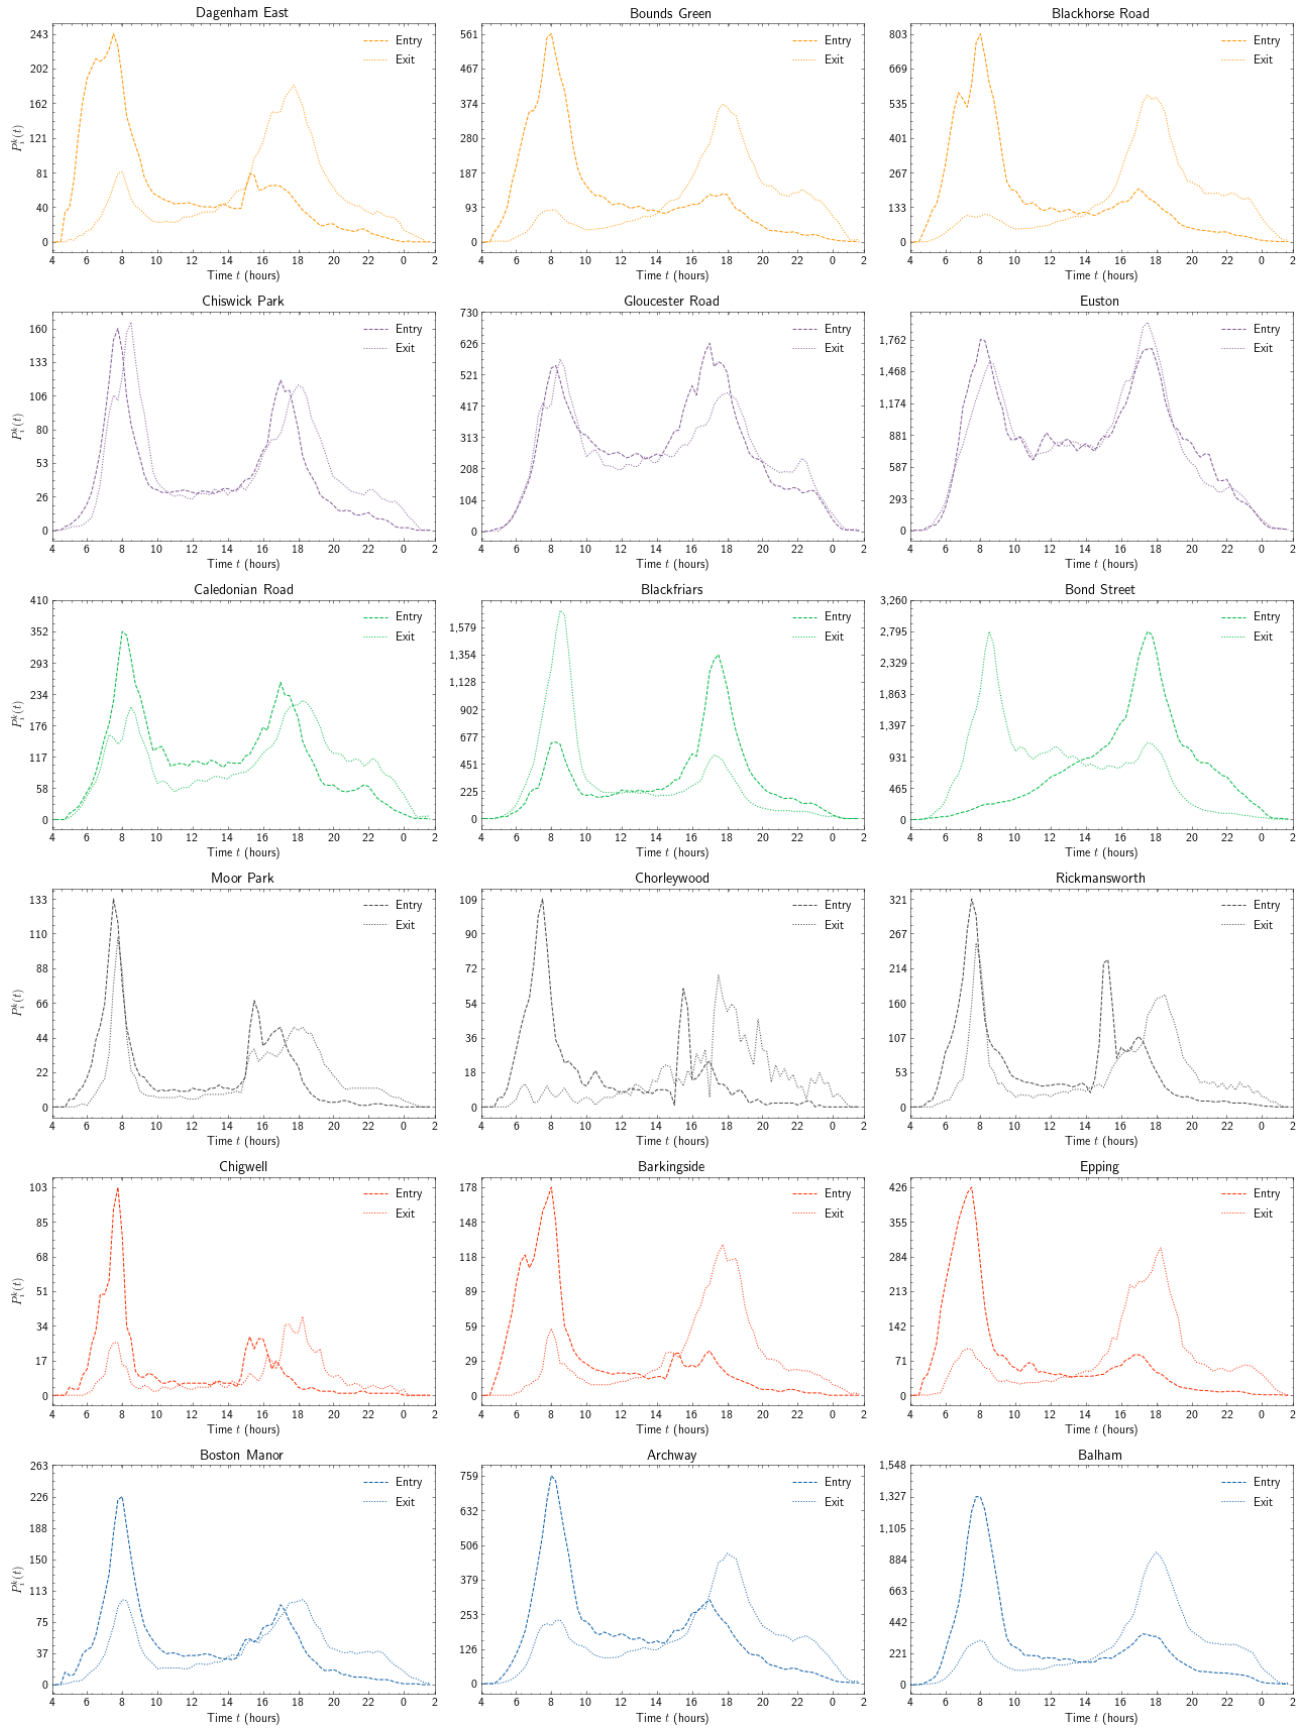

Supplementary Fig. 1. **An overview of the station traffic in Greater London.** Passenger counts  $P_i^k(t)$  showing entrances for every 15-minute intervals for stations in different clusters of the PT system. Each row is a cluster that a station belongs to (from top to bottom: inner-residential, polycentre, CBD, mixed commuter, outer-residential, potential feeder). Each column is an example of station traffic (from left to right: low, medium and high traffic).

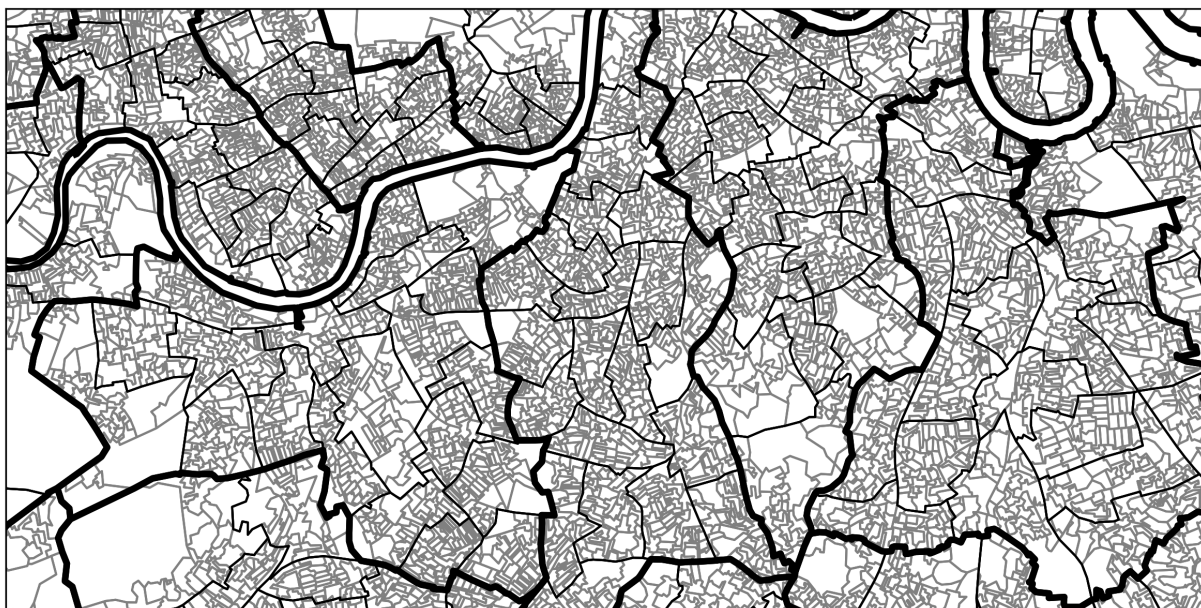

Supplementary Fig. 2. **Census estimate area of Greater London.** Portion of London showing Output Areas (thin gray lines), wards (thin black lines), and boroughs (thick black lines) in order of decreasing resolution.

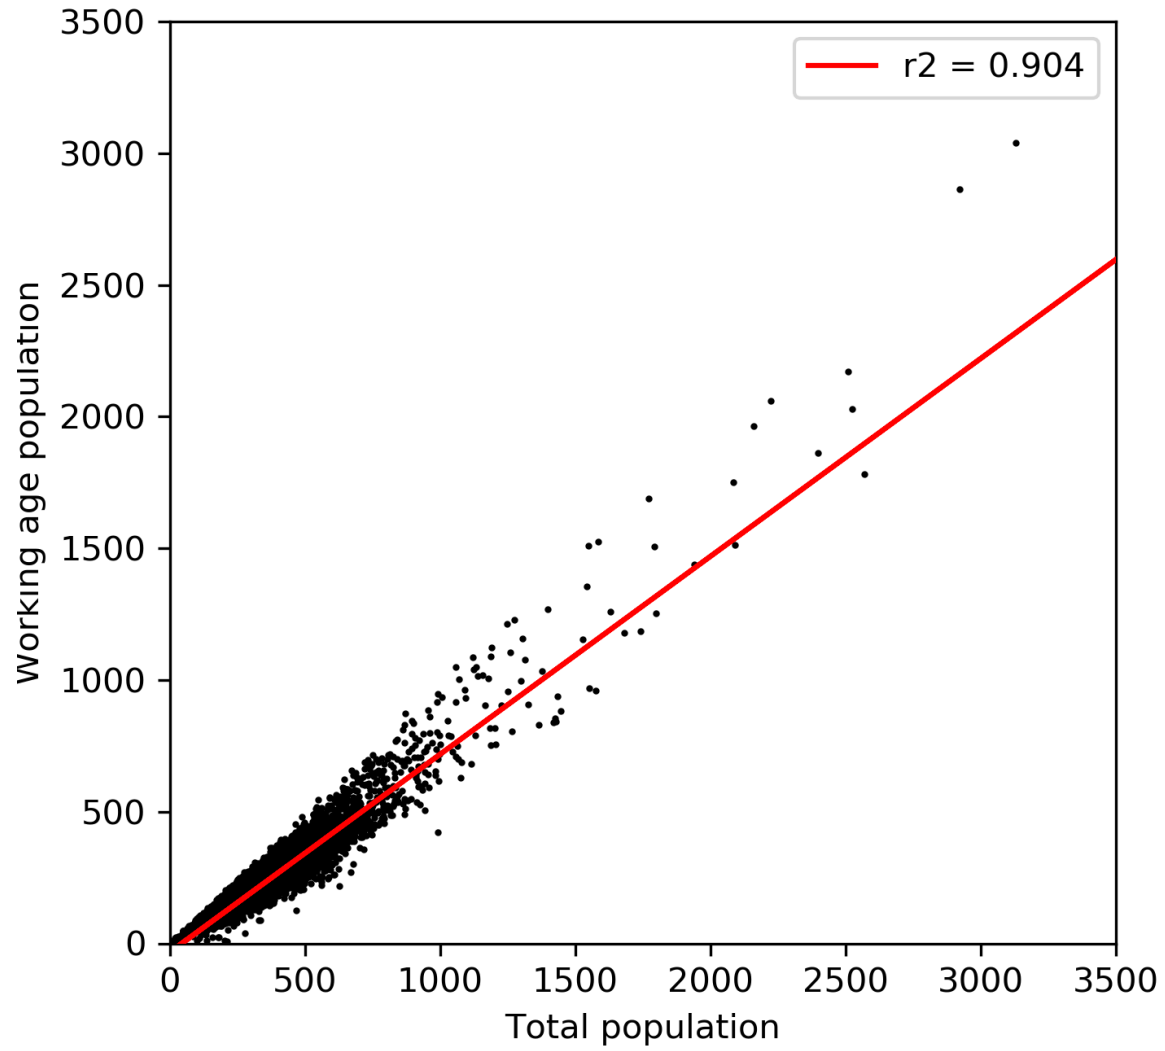

Supplementary Fig. 3. **Comparison of census population statistics.** Working-age population compared to total population for all Greater London Output Areas. Each point is an output area and the population estimates are gathered from Ref. [1].

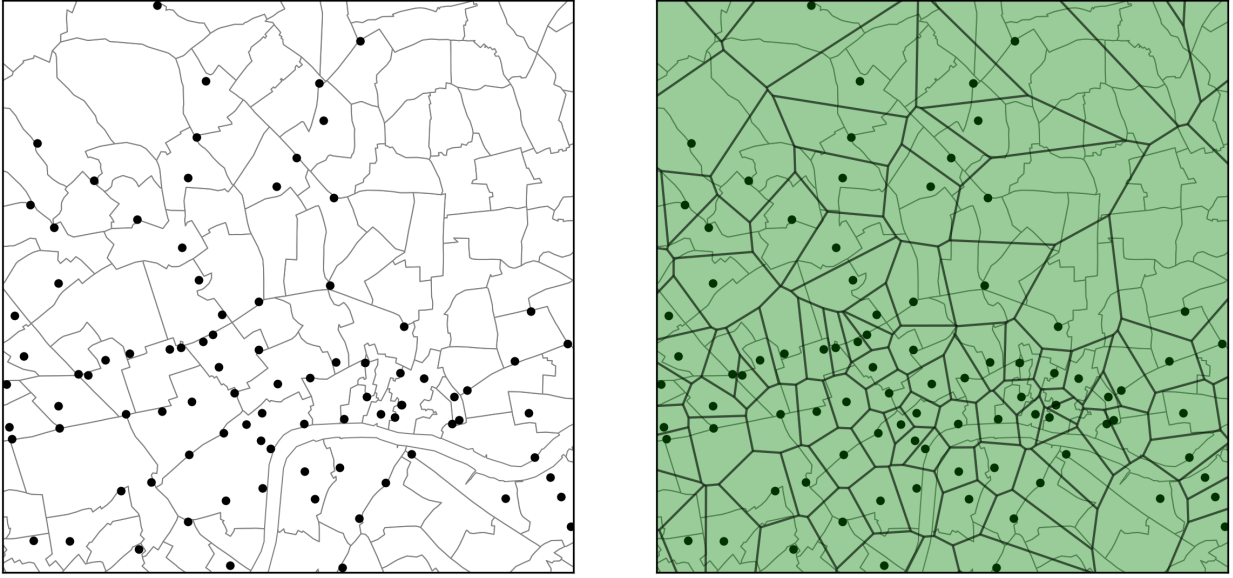

Supplementary Fig. 4. **Station Voronoi Zones.** A portion of Greater London is shown here. (left) Locations of stations. (right) Voronoi cells measured around each station. Every point in a cell is closer to the station within the cell than stations outside the cell.

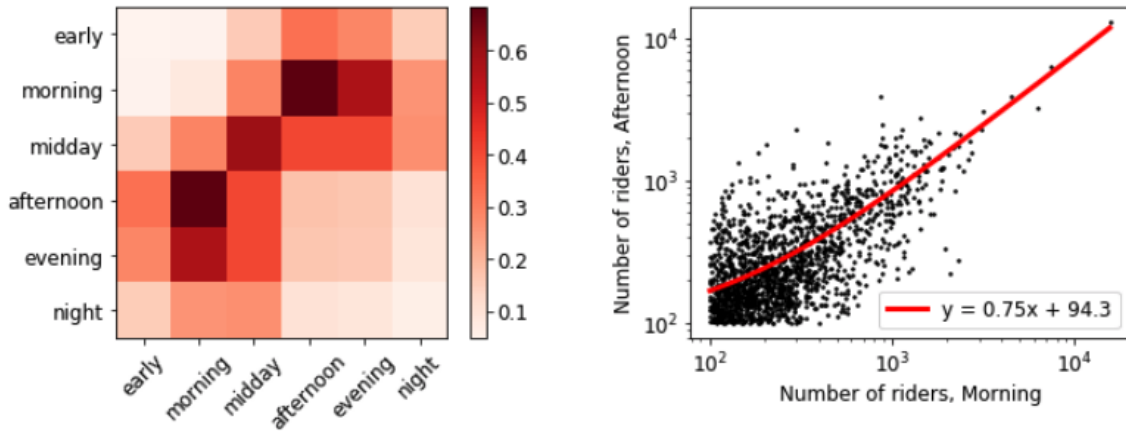

Supplementary Fig. 5. **Symmetry between morning and afternoon ridership.** (left) Correlation between trips in opposite directions for different times of day. For example, the bottom left square represents the correlation between trips made in one direction (e.g. from station  $i$  to station  $j$ ) at night and in the opposite direction (from station  $j$  to station  $i$ ) in the early morning. (right) Number of trips between pairs of stations in the morning and in the opposite direction in the afternoon, for routes with more than 100 riders in each direction. Each point represents a pair of stations from the RODS data. The time categories in the left frame have not been derived from the six demand profiles. 16 time slots are aggregated into one bin for simplicity.

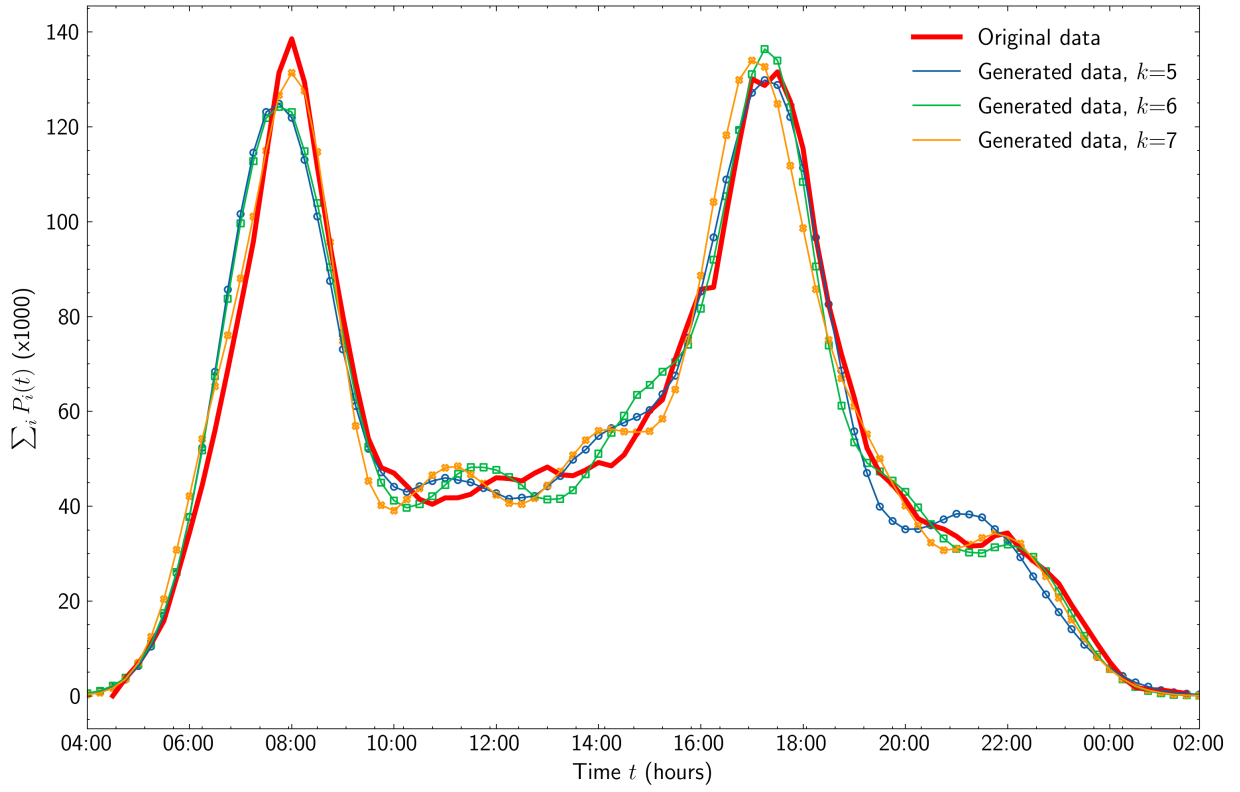

Supplementary Fig. 6. **Demand profile variation.** Total station traffic  $\sum_i P_i(t)$  for the PT system showing entrances for every 15-minute intervals. The thick red line shows the original data. The other three lines (blue ( $k = 5$ ), green ( $k = 6$ ) and yellow ( $k = 7$ )) show generated station traffic using the GMM that we formulated. The plot shows that there is very little deviation from the original station traffic data for all demand profile sizes (5, 6, and 7). As data is underdispersed in certain time intervals, there is some loss in accuracy (see Supplementary Note 4).

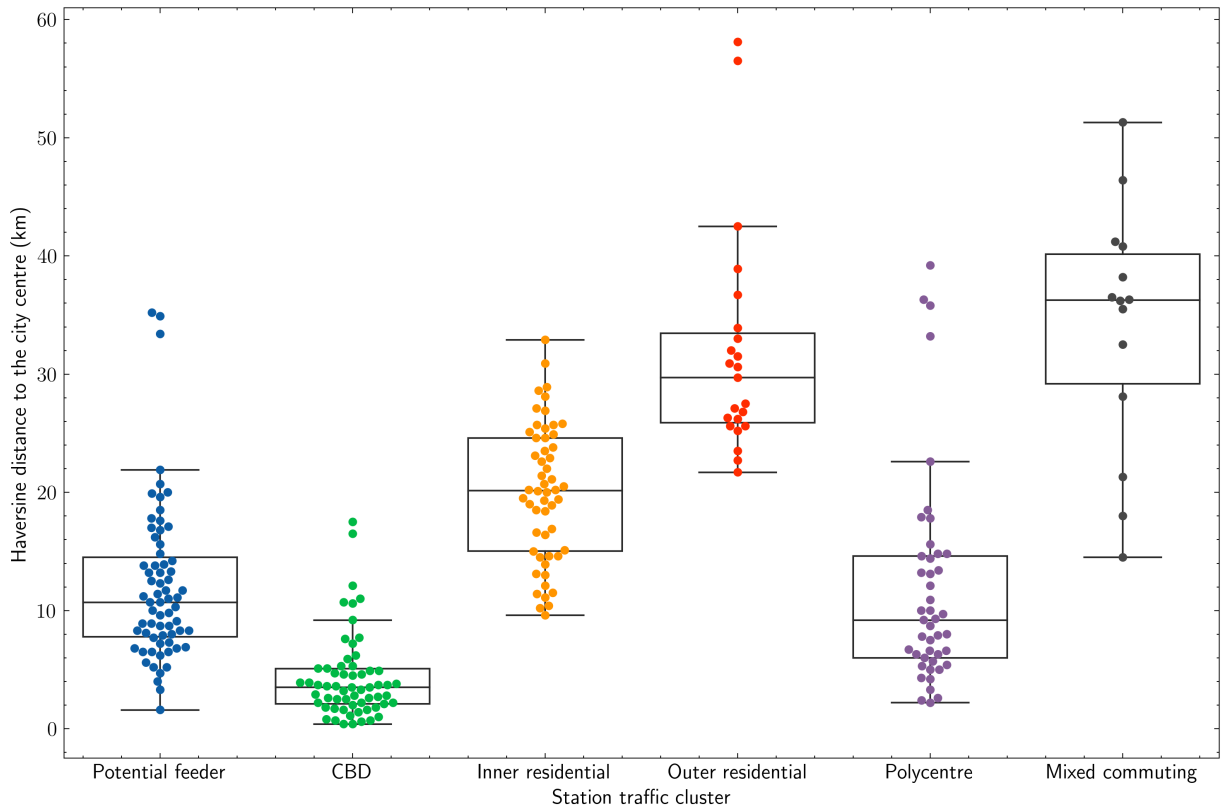

Supplementary Fig. 7. **Box-plot representation of distance to the city centre for different clusters.** The distance values of each station from the city centre shown in the box-plots for different station clusters is measured using the Haversine distance formula [2]. The points are shown for visual representation of the distributions. The black line inside each box shows the median distance for each cluster distribution and the whiskers are chosen to show 1.5 of the interquartile range. The coordinates of the centre of the city were chosen as  $(51.5074, -0.1278)$  which corresponds to Trafalgar Square.

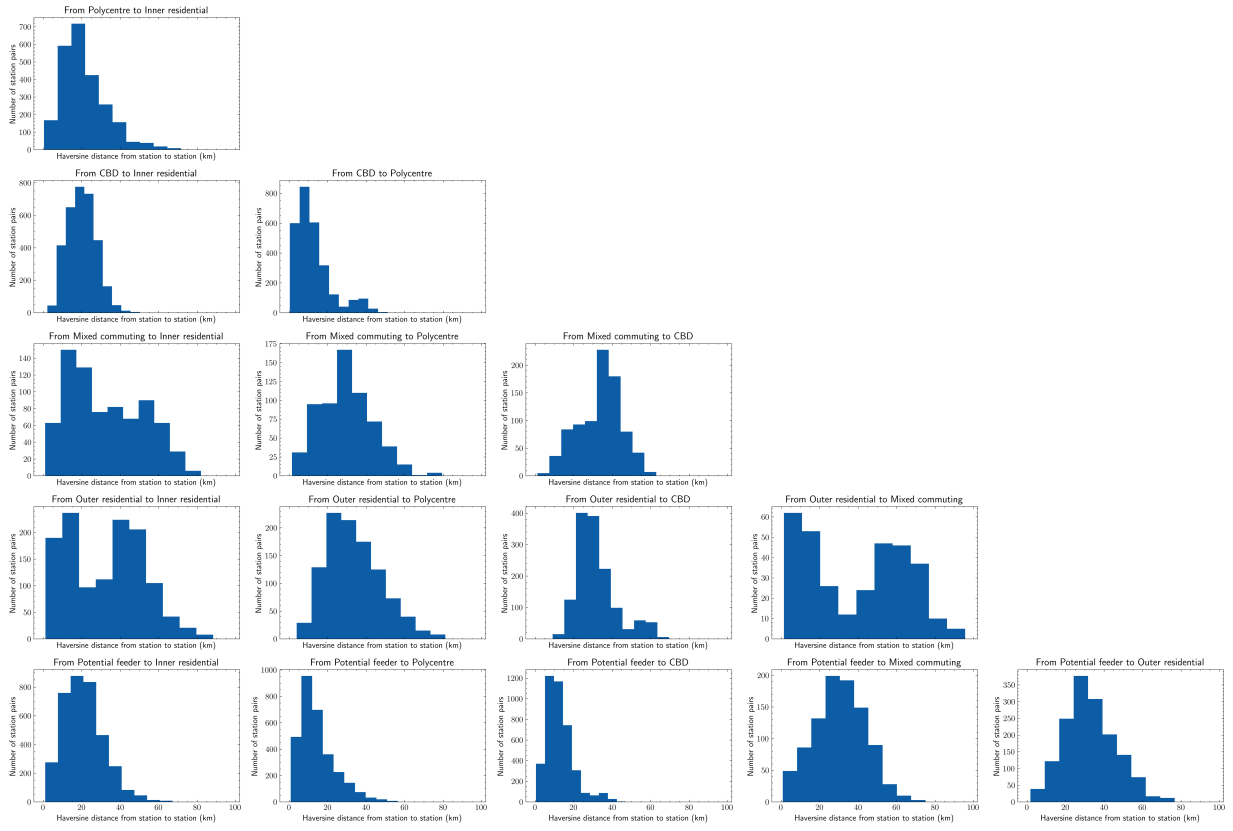

Supplementary Fig. 8. **Distribution of distances between cluster stations.** The lower triangular matrix showing Haversine distance distribution between each pair of clusters. Each plot shows the frequency of inter-cluster stations for increasing Haversine [2] distance.

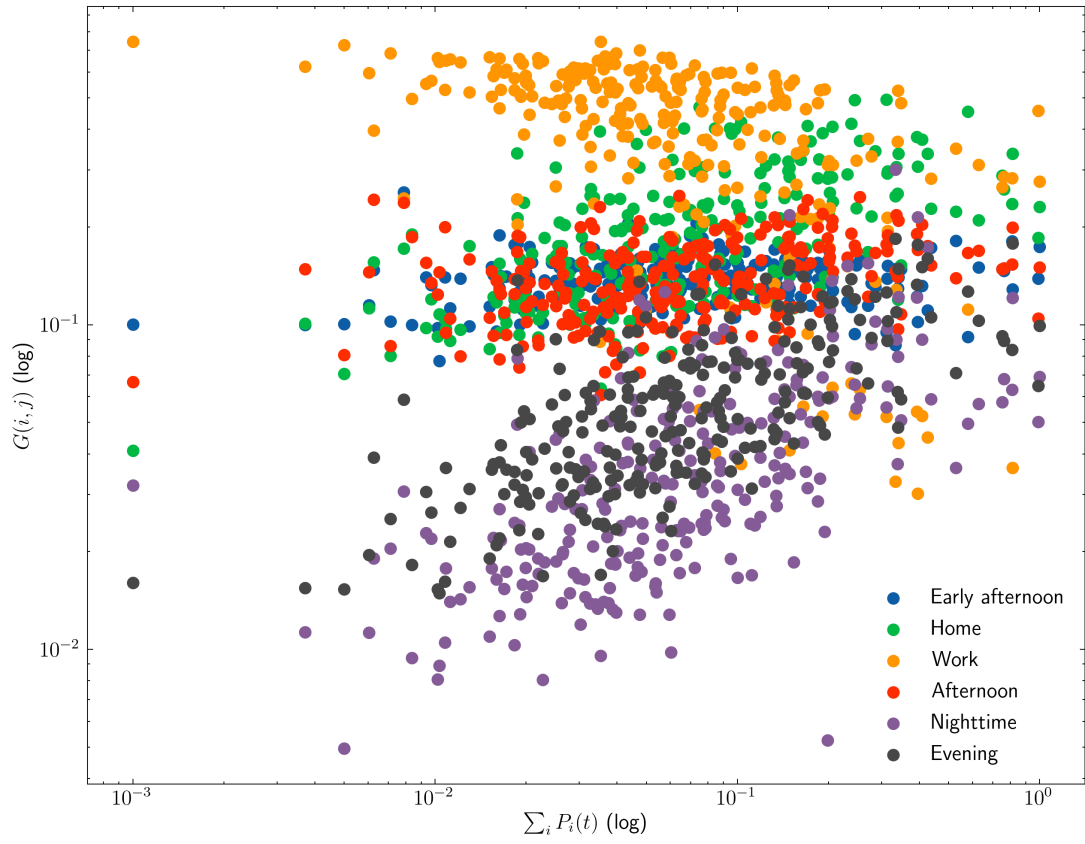

Supplementary Fig. 9. **Likelihood of stations serving a demand profile.** Log-Log scatter plot of likelihood of stations serving a demand profile type,  $G(i, j)$ , versus total number of entrances per station,  $\sum_i P_i(t)$ , scaled between 0 and 1. The likelihoods  $G(i, j)$  sum to 1 for all values of profile  $j$ . Different colours represent the demand profiles.

## SUPPLEMENTARY NOTE 1: STATION ZONE ESTIMATION

### Census data

Part of our analysis involves comparing the ridership to the population within the regions surrounding the station. We therefore require high-resolution data of the London population. For this, we use the official 2017 Census Output Area estimates [1]. Output Areas are the smallest census designation in the UK (Fig. 2), providing us with the highest resolution population estimates possible. This high resolution allows us to aggregate the census areas in order to estimate the population within each station zone. Although the 2017 census is only an estimate <sup>1</sup>, it provides a better approximation of the existing London population compared to the full census performed in 2011, which is outdated for an analysis in the year 2017.

The census population estimate is divided by age. Since we focus on identifying demand profiles and their relationship to population statistics, we restrict the census population to the working age population which we designate as ages between 18 and 65 (the number of children and older adults who do may use the public transport at all, may skew the relationship). There is a strong correlation between the working-age population and the total population (Fig. 3), which indicates that our analysis is robust to the age range that we use.

### Station population zones

To measure the population of every station zone, we designate station zones as Voronoi tessellations (all points in a zone are close to the designated station than any other station). Then we assume all entrances to a station are attributed to the population residing within a station's zone as the transit riders will enter the station that is closest to them (Fig. 4).

### Accessibility Analysis

Given that not every person entering a station is necessarily located within a station's zone, our correlation analysis for station accessibility is simplified. Though, this is not the main research question, we address a few problems with the data we have and provide a possible path for the future in case that level of resolution becomes available.

First, passengers may connect at a station via other modes of transport such as private vehicles, bicycles, buses, and overground rail. Under our assumption, passengers coming from completely different areas (for example, by walking or via bus transit) would still be considered as living or working near a station simply because they connect with that station during their daily commute. Second, we do not consider the transit lines to which the stations belong. Given a choice between two stations, the assumption that passengers will enter the station closest to them is reasonable when both stations are part of the same transit line, but when each station belongs to different lines, or to multiple lines, this assumption is no longer valid. For example, a passenger may be located 200m from one station on Line A and 400m from another station on Line B. Both stations are walking distance and depending on convenience, a passenger may enter either station. However, under our accessibility model, we assume the passenger will enter the station located on Line A because it is closer.

By regressing ridership against population  $P_i(t) = \alpha p_i$ , where  $p_i$  is the residential population within the station zone, and  $\alpha$  is a proportionality constant, our baseline suggests that passengers enter the station that they live nearest to and a proportion ( $\alpha$ ) of residents using the underground network in Greater London (compared to other modes of transport) is constant across all stations. Passengers entering a station may come from far away, having walked or used other modes of private transport to get to their desired station, biased by the complexity of the trip and their mode choice [3] or friendliness of the built environment [4]. Moreover, the proportion of passengers using the transport system is known to depend heavily on socioeconomic factors [5], and therefore is not constant across all stations situated in different urban neighbourhoods. A potential implication of these limitations in the data may be responsible for the over- and underestimations of the regressions.

To interpret station-cluster-specific regression errors, we define a theoretical model which could potentially draw out features that explain ridership at any particular station:

$$P_i(t) = \alpha_s p + p_{fromElsewhere} - p_{toElsewhere}, \quad (1)$$

---

<sup>1</sup> This method uses change in the population recorded in administrative sources as an indicator of change in the true population, and it is used to produce estimates in intercensal periods.

where  $\alpha_s$  is the station-specific proportion of the residential population using the transit network,  $p_{fromElsewhere}$  is the number of passengers coming from areas outside the zone in order to enter the station, and  $p_{toElsewhere}$  is the number of passengers leaving their zone to go to another station. To account for the errors, we could measure the difference between the two models:

$$\epsilon_i = p_{fromElsewhere} - p_{toElsewhere} + (\alpha_s - \alpha_{mean})p. \quad (2)$$

Thus, the error would represent some critical properties of the transport system. A large positive error can represent one of two things: a large number of riders coming from other areas, or a larger than expected percentage of inhabitants taking the train (deviation from the mean). On the other hand, a large negative error represents the opposite: many inhabitants taking the train somewhere else, or fewer than expected inhabitants taking the train at all. Essentially, the error in the regression could measure how well the station performs or how well two modes are tied together (for example, feeder buses dropping passengers at well-performing stations).

A future direction for investigation could thus be to measure zonal population movements preceding the use of transport service and how the vector of  $\epsilon$ s maps to a measurement of attraction to a location in time (for example, a weighted amenities and points of interest analysis). If such population movement surveys become available, our method can be adapted easily.

## SUPPLEMENTARY NOTE 2: ROLLING ORIGIN-DESTINATION SURVEY DATA

For understanding the correctness and potential value of the Automatic Fare Collection (AFC) [6] data set, we perform statistical tests using Origin-Destination (OD) matrices from RODS [7] that are representative of flows in the system. The daily morning and afternoon commutes have some degree of symmetry, pointing to regular residential and work demand profiles where trips in one direction in the morning are accompanied by approximately the same amount of trips in the opposite direction in the afternoon. The RODS dataset describes the number of trips between all stations, provided as origin-destination pairs. The trips are for weekdays only and are according to the time of day. Like the Passenger Counts, the RODS is based on rides in November of 2017. Though the AFC and the RODS data sets are similar, the former excludes trips made on other networks sharing the station (e.g. National Rail and Bus services) and the latter only represents 5% of the population.

We can examine the symmetry by calculating the correlation coefficient between opposing trips during different time periods (Fig. 5). As expected, we see that the strongest symmetry occurs between morning and afternoon trips, followed by a symmetry between morning and evening trips. This suggests that commuting trips are highly symmetric: people who go to work in the morning take the same way to get back home in the afternoon. Our primary analyses is based on AFC, while the RODS data set is used to establish the correctness of using entry-only information and substantiating the complexity of the urban demand.

It is notable that the morning and afternoon routes are not just symmetric, but also represent the dominant form of mobility taking place on the transit network, in terms of sheer numbers. However, in the RODS data set, symmetric and regular (work and residential) ridership represent 47% of all trips taking place on a weekday, which is less than half of all trips on the network. Often, in this dominating statistic, other profiles of ridership are ignored, hence it is important to look at demand profiles across a day.

## SUPPLEMENTARY NOTE 3: DIFFERENCES IN URBAN TRANSPORT PLANNING FOR VARIOUS STATION CLUSTERS.

To interpret differences in station use, we calculate the likelihood that a station  $i$  is of demand profile type  $j$ ,

$$G(i, j) = \frac{1}{N_i} \sum_{x(t)} p(C_j | x(t)). \quad (3)$$

$N_i$  is the cumulative number of users entering a station  $i$  on a representative day.  $x(t)$  accounts for all data points at every time-step for a particular station and  $\sum_j G(i, j) = 1$  for all stations. Figure 9 shows as the size of total traffic at a station increases, we see a convergence in demand profiles toward mixed-use. Smaller stations are much more likely to serve only one kind of demand which is workbound. Larger outlier stations like Waterloo, Brixton and Stratford are considered mixed-use because these stations also serve other modes of transportation like national rail, overground, DLR and large bus hubs. Thus, looking at the convergence of likelihoods  $G(i, j)$  of station traffic it is possible to differentiate station outliers from large urban hubs having several businesses, residences and amenities.

# SUPPLEMENTARY NOTE 4: DATA LIMITATIONS

We make a number of assumptions in our study concerning traffic (Table II). In the following paragraphs we systematically examine these assumptions, consider their validity, and evaluate the consequences should these assumptions be violated.

The model is certainly heterogeneous across the days of the week, and across seasons of the year, thereby violating one of the model assumptions. A more complete model would better enable tracking of consumers and of tourists, who characteristically swell numbers on the rail during the weekends and summer months. If this data were incorporated in the model, an even more differentiated profile of the stations may emerge as a result. Hints of this phenomena are seen in the data, with evidence of polycentric patterns around the margins of Greater London. Nonetheless this assumption of traffic homogeneity does not invalidate the results demonstrated for a sample of passengers using the system during weekdays and winter months, as these use cases are separable in time and space.

The model should certainly be better conditioned on the available connections at the station. These conditional patterns can be seen in the main text Fig. 3, where stations have been clustered by their characteristic traffic patterns. The revealed station types show a strongly concentric character, with one type of station predominating in the centre, and other types predominating at the periphery. In fact, these station types probably confound to different phenomena – the district type, as well as the commuter type of station. Nonetheless, it is also entirely consistent with urban theory that residential and business development should also follow such a concentric pattern around the city centre. One station in particular, Euston Station, stands out as especially unusual in its traffic patterns. These unusual patterns may well result from the role of the station as part of a multi-modal transportation hub.

The model assumptions of conditional independence given six mixtures holds up well to the data. Tests of robustness are performed for a range of different mixtures ranging from five to seven, and these characteristic patterns remain, albeit with varying levels of detail and stability concerning the mid-afternoon traffic. The data is non-Gaussian in two specific ways, neither of which challenge the validity of the model. The first potential challenge has to do with boundary effects as the stations open and closes. The peak morning hours and evening hours are far enough away from opening and closing times that the empirical distribution is not truncated at the margins. The empirical distribution is under-dispersed, with people bunching up to use stations at rush hours such as noon and six. Our investigations demonstrate that the peaks constitute only a modest additional passenger flow above and beyond the underlying Gaussian distribution. Furthermore, the additional empirical peak is symmetrical around the rush hours (main text Fig. 1); it therefore causes only minor challenges to estimation: causing an underestimation of the tails of the traffic demand.

Supplementary Table I. Statistical properties of the *six* demand profiles:  $\mu$ ,  $\sigma$  and  $\phi$ .

| Demand Profiles      | $\mu$ | $\sigma^2$ | $\phi$ |
|----------------------|-------|------------|--------|
| Early afternoon (EA) | 40.11 | 5.49       | 0.14   |
| Residential (R)      | 62.96 | 3.51       | 0.24   |
| Work (W)             | 24.55 | 4.56       | 0.31   |
| Afternoon (A)        | 53.72 | 4.63       | 0.15   |
| Nighttime (N)        | 82.37 | 3.89       | 0.06   |
| Evening (E)          | 72.43 | 3.84       | 0.09   |

Supplementary Table II. Model Assumptions and Validity

| Class of Assumptions | Specific Label              | Degree of concern                                                                                             |
|----------------------|-----------------------------|---------------------------------------------------------------------------------------------------------------|
| Traffic modelling    | Volume                      | Minor                                                                                                         |
| Temporal modelling   | Gaussian                    | Investigations in demonstrate the departures from Gaussian are comparatively minor (SN4)                      |
|                      | Homogeneous across week     | Potentially concerning, but does not invalidate the core findings as they are related to traffic across a day |
|                      | Homogeneous across year     | Potentially concerning, but does not invalidate the core findings as they are related to traffic across a day |
| Spatial modelling    | Independent of district     | District-level effects are subsumed in the mixture weights                                                    |
|                      | Independent of connection   | Risks compounding network connections with underlying district type or use                                    |
| Environmental        | Independent of weather      | Minor, given the extensive character of the sample                                                            |
|                      | Independent of road traffic | Minor, since systematic variations in demand are measured by the data                                         |

- 
- [1] Census Output Area population estimates – London, England.
  - [2] Charles H. Cotter. *A history of nautical astronomy*. Hollis & Carter, London, Sydney [etc.], 1968.
  - [3] Lawrence Frank, Mark Bradley, Sarah Kavage, James Chapman, and T. Keith Lawton. Urban form, travel time, and cost relationships with tour complexity and mode choice. *Transportation*, 35(1):37–54, January 2008.
  - [4] Robert Cervero and Jin Murakami. Effects of Built Environments on Vehicle Miles Traveled: Evidence from 370 US Urbanized Areas. *Environment and Planning A: Economy and Space*, 42(2):400–418, February 2010.
  - [5] John Holtzclaw, Robert Clear, Hank Dittmar, David Goldstein, and Peter Haas. Location Efficiency: Neighborhood and Socio-Economic Characteristics Determine Auto Ownership and Use - Studies in Chicago, Los Angeles and San Francisco. *Transportation Planning and Technology*, 25(1):1–27, January 2002.
  - [6] London Underground passenger counts data.
  - [7] Rolling Origin & Destination Survey (RODS).
